# Supplementary material for: StyTr$^2$: Image Style Transfer with Transformers
Source: arXiv:2105.14576 source file (2022-04-01)
Supplement: Supplementary file 1 [file fig_supp_weights.tex]

% \begin{figure}%[!h]
% \setlength{\abovecaptionskip}{0mm}
% \centering
% \includegraphics[width= \linewidth]{image/weight.pdf}
% \caption{Impact of style weight.
% }
% \label{fig:weight}
% \end{figure}

\newcommand\weightfigurewidth{0.24}

\begin{figure}%[b]
\setlength{\abovecaptionskip}{2mm}
\centering
\includegraphics[width=\weightfigurewidth\linewidth]{image/figs_weight/c1.png}
\includegraphics[width=\weightfigurewidth\linewidth]{image/figs_weight/wl1.png}
\includegraphics[width=\weightfigurewidth\linewidth]{image/figs_weight/wh1.png}
\includegraphics[width=\weightfigurewidth\linewidth,height=\pecomparisonfigurewidth\linewidth]{image/figs_weight/s1.png}

\includegraphics[width=\weightfigurewidth\linewidth]{image/figs_weight/c2.png}
\includegraphics[width=\weightfigurewidth\linewidth]{image/figs_weight/wl2.png}
\includegraphics[width=\weightfigurewidth\linewidth]{image/figs_weight/wh2.png}
\includegraphics[width=\weightfigurewidth\linewidth,height=\pecomparisonfigurewidth\linewidth]{image/figs_weight/s2.png}

\begin{minipage}{\weightfigurewidth\linewidth}
    \centering
    \figtext{Content}
\end{minipage}
\begin{minipage}{\weightfigurewidth\linewidth}
    \centering
    \figtext{$\lambda_{s} = 5$}
\end{minipage}
\begin{minipage}{\weightfigurewidth\linewidth}
    \centering
    \figtext{$\lambda_{s} = 10$}
\end{minipage}
\begin{minipage}{\weightfigurewidth\linewidth}
    \centering
    \figtext{Style}
\end{minipage}
\caption{Impact of style weight.
}
\vspace{-2mm}
\label{fig:weight}
\end{figure}
