# Supplementary material for: StyTr$^2$: Image Style Transfer with Transformers
Source: arXiv:2105.14576 source file (2022-04-01)
Supplement: Supplementary file 2 [file fig_supp_ItoS.tex]

% \begin{figure}%[!ht]
% \setlength{\abovecaptionskip}{2mm}
% \centering
% \includegraphics[width= \linewidth]{image/ItoS2.pdf}
% \caption{Comparisons of CNN and Linear projection through several rounds of image stylization.
% }
% \label{fig:ItoS2}
% \end{figure}

\newcommand\Ttosfigurewidth{0.22}
\newcommand\Ttostextwidth{0.015}

\begin{figure}%[b]
\setlength{\abovecaptionskip}{2mm}
\centering

\begin{minipage}{\Ttostextwidth\linewidth}
    \centering
    \rotatebox{90}{\figtext{Style}}
\end{minipage}
\hspace{0pt}
\begin{minipage}{\Ttosfigurewidth\linewidth}
    \includegraphics[width=\linewidth]{image/figs_ItoS2/s.png}
\end{minipage}
\begin{minipage}{\Ttosfigurewidth\linewidth}
    \includegraphics[width=\linewidth]{image/figs_ItoS2/l1.png}
\end{minipage}
\begin{minipage}{\Ttosfigurewidth\linewidth}
    \includegraphics[width=\linewidth]{image/figs_ItoS2/l2.png}
\end{minipage}
\begin{minipage}{\Ttosfigurewidth\linewidth}
    \includegraphics[width=\linewidth]{image/figs_ItoS2/l3.png}
\end{minipage}
\begin{minipage}{\Ttostextwidth\linewidth}
    \centering
    \rotatebox{90}{\figtext{Linear}}
\end{minipage}

\begin{minipage}{\Ttostextwidth\linewidth}
    \centering
    \rotatebox{90}{\figtext{Content}}
\end{minipage}
\hspace{0pt}
\begin{minipage}{\Ttosfigurewidth\linewidth}
    \includegraphics[width=\linewidth]{image/figs_ItoS2/c.png}
\end{minipage}
\begin{minipage}{\Ttosfigurewidth\linewidth}
    \includegraphics[width=\linewidth]{image/figs_ItoS2/cnn1.png}
\end{minipage}
\begin{minipage}{\Ttosfigurewidth\linewidth}
    \includegraphics[width=\linewidth]{image/figs_ItoS2/cnn2.png}
\end{minipage}
\begin{minipage}{\Ttosfigurewidth\linewidth}
    \includegraphics[width=\linewidth]{image/figs_ItoS2/cnn3.png}
\end{minipage}
\begin{minipage}{\Ttostextwidth\linewidth}
    \centering
    \rotatebox{90}{\figtext{CNN}}
\end{minipage}

\begin{minipage}{\Ttosfigurewidth\linewidth}
    \centering
    \figtext{Input}
\end{minipage}
\begin{minipage}{\Ttosfigurewidth\linewidth}
    \centering
    \figtext{Round 1}
\end{minipage}
\begin{minipage}{\Ttosfigurewidth\linewidth}
    \centering
    \figtext{Round 2}
\end{minipage}
\begin{minipage}{\Ttosfigurewidth\linewidth}
    \centering
    \figtext{Round 3}
\end{minipage}
\caption{Comparisons of CNN based and our linear projection based layers through several rounds of image stylization.
}
\vspace{-2mm}
\label{fig:ItoS2}
\end{figure}
