# Supplementary material for: StyTr$^2$: Image Style Transfer with Transformers
Source: arXiv:2105.14576 source file (2022-04-01)
Supplement: Supplementary file 5 [file fig_supp_progressive.tex]

\newcommand\pecomparisonfigurewidth{0.24}

\begin{figure}%[b]
\setlength{\abovecaptionskip}{2mm}
\centering
\includegraphics[width=\pecomparisonfigurewidth\linewidth,height=\pecomparisonfigurewidth\linewidth]{image/figs_progressive/c.PNG}
\includegraphics[width=\pecomparisonfigurewidth\linewidth]{image/figs_progressive/single.PNG}
\includegraphics[width=\pecomparisonfigurewidth\linewidth]{image/figs_progressive/m.PNG}
\includegraphics[width=\pecomparisonfigurewidth\linewidth,height=\pecomparisonfigurewidth\linewidth]{image/figs_progressive/s.PNG}

\begin{minipage}{\pecomparisonfigurewidth\linewidth}
    \centering
    \figtext{Content}
\end{minipage}
\begin{minipage}{\pecomparisonfigurewidth\linewidth}
    \centering
    \figtext{Single-layer}
\end{minipage}
\begin{minipage}{\pecomparisonfigurewidth\linewidth}
    \centering
    \figtext{Multi-layer}
\end{minipage}
\begin{minipage}{\pecomparisonfigurewidth\linewidth}
    \centering
    \figtext{Style}
\end{minipage}

\caption{The impact of progressive generation of transformer decoder.
}\label{fig:progressive}
\end{figure}
