# Supplementary material for: StyTr$^2$: Image Style Transfer with Transformers
Source: arXiv:2105.14576 source file (2022-04-01)
Supplement: Supplementary file 6 [file tab_supp_progressive.tex]

\begin{table}%[!h]
\small
\setlength\tabcolsep{2.5pt}
\centering
\begin{tabular}{c|cc}
\toprule
&Single-layer &Ours (multi-layer)  \\
\midrule
$\contentloss$ $\downarrow$ & 1.94& \textbf{1.91} \\
$\styleloss$ $\downarrow$ & 2.38 & \textbf{1.47}  \\
\bottomrule
\end{tabular}
\vspace{-5pt}
\caption{Quantitative evaluation of progressive generation.}
\label{tab:loss1}
\end{table}
